# Supplementary material for: ATM: Action Temporality Modeling for Video Question Answering
Source: arXiv:2309.02290 source file (2023-09-05)
Supplement: Supplementary file 1 [file 6-supplementary.tex]

In this document, we provide additional analysis of \methodname. All of the details and analyses we included in this document were ready at the time of submission but were not included in the main paper due to the page limit.

\section{Implementation Details}
\textbf{Text Features}
A pre-trained language model BERT \cite{devlin2018bert} was used to extract text embedding of questions and answers. Based on previous work \cite{xiao2022vgt}, we concatenate a question and its corresponding candidate answer as a QA pair in the multiple-choice QA task as the input of text feature extraction. For the open-ended QA task, questions and answers are processed separately. A linear layer is used to encode the text features into the visual-language space.

\textbf{Multi-stream Video Encoder (MSVE)} In Sec.3.1 and 3.2, we extract video representation by a multi-stream video encoder that fuses the three streams \ie object-level, frame-level appearance, and motions. Feature extraction for the three-stream input has been explained in Sec 4.2. The feature extraction is performed offline without parameters finetuning, due to the limitation of computation resources. 
We further apply the dynamic graph transformer(DGT) proposed by the state-of-the-art (SoTA) method VGT~\cite{xiao2022vgt} to encode the object relations and get the object representation $f_o$, to make a fair comparison with SoTA.  
For RGB frames and optical flow features, we linearly encode them to $f_i$ and $f_m$. The feature dimension of $f_o,f_i,f_m$ are all $512$-d. Then, we aggregate the three streams by concatenating the three features as per each timestamp and encode them into $512$-d by an MLP layer. 
After that, the MSVE contains a multi-head self-attention layer (MSA) with a learnable sinusoidal temporal position embedding~\cite{devlin2018bert} to capture the inter-frame dynamics. The number of heads is set as $8$. The dimension of the hidden states in MSA is also $512$.

\textbf{Temporal Sensitivity-aware Confusion Loss}
English questions typically follow a syntactic structure. Temporal-sensitive questions contain specific syntax, \eg ``after'', ``before'', ``... when...", ``...while...'' and \etc. The remaining is descriptive questions, \eg a count question, \textit{``How many people are involved in the video?''}, which is insensitive to time. 
We detect the existence of the syntaxes and filter out the temporal-insensitive questions. 
For Next-QA, we have $17,681$ temporal-sensitive questions and $16,451$ temporal-insensitive questions in the training set.
For T-Gif~\cite{li2016tgif}, as its ``action'' and ``transition'' splits focus on repeated actions and transitions respectively, all of the questions in those splits are temporally sensitive. 
For the open-ended QAs including TGif-FrameQA and MSRVTT~\cite{xu2016msr}, we do not apply the confusion loss as they focus more on the descriptive content.

\textbf{Action Phrase}
We parse the action phrases from questions using SpaCy parser~\cite{spacy2} Specifically, we use dependency parsing to get the phrases in a question and use the pos-tag to find the verb in the question. Then we filter the phrases that contain the verb and select the shortest one as the action phrase. For example, for the question ``what happens to the train after moving for a while near the end?'', the action phrase is ``moving for a while''.

\begin{figure*}
    \centering
    \includegraphics[width=0.9\textwidth]{figures/visual_supp2.pdf}
    \caption{\textbf{Visualization.} The ground-truth is marked in green. We display the representative result and failure case of ATM, ATM w/o AcCL (as “Ours w/o AcCL”), ATM w/o motion stream (as “Ours w/o mot”), and the existing SoTA method VGT.}
    \label{fig:visual_supp}
\end{figure*}

\textbf{Open-Ended QA Setting}
Following VGT, text encoder $\mathcal{F}_q\left (\cdot \right )$ takes question-answer pair $[q;a]$ as input (see Eq.2 in the main paper) for multiple-choice QA (MC-QA) and takes answer $a$ as input for open-ended QA (OE-QA). To integrate the question information in OE-QA, we add a cross-modal interaction (CI) proposed by VGT to enhance video representations with question information as $f_{qv}$. (See VGT's Sec 3.4 for the details of CI). For OE-QA, Eq.4 in the main paper is modified as:
% into the video representation as $f_{qv}$ 
\begin{equation}
f_{qv} = \text{MPool}(\text{CI}(\text{MSA}(\text{MLP}([f_o ; f_i ; f_m]))),\mathcal{F}_q \left (q\right ) ).
\label{oe_fv}
\end{equation}
In VGT, cross-modal interaction is applied for both MC-QA and OE-QA. But we realize that the cross-modal interaction is not apparently helpful in the MC-QA, thus we only keep it for OE-QA.

Following VGT, we enable a joint decision between video-included and video-absent QA for open-ended setting, which modifies Eq.2 of the main paper as:
\begin{equation}
  s_a = f_{qv} \mathcal{F}_q \left (a\right )^\top \odot  \mathcal{F}_q \left (q\right ) \mathcal{F}_q \left (a\right )^\top,
\label{oe_sim}
\end{equation}
where $\mathcal{F}_q \left (q\right ) \mathcal{F}_q \left (a\right )^\top$ simply computes the cosine similarity between the question and the answer.

\section{Additional Quantitative Analysis}
\input{tables/comparison_tgif_frameqa}
\subsection{TGIF-FrameQA}
Following the SoTA~\cite{xiao2022vgt}, we compare ~\methodname with previous work on the FrameQA split in Table~\ref{tab:frameqa}, as well as TGIF's transition and actions splits in Table 2 of the main paper. It shows that our method performs close to the pretraining-free SoTA VGT~\cite{xiao2022vgt}. Large-scale pretraining method MERLOT~\cite{zellers2021merlot} achieves the best performance on the FrameQA split. This is because the FrameQA split has a lot of descriptive questions that can be answered from a single frame, where good pretraining is helpful. 
This demonstrates that although \methodname focuses on temporal reasoning, the representation of descriptive content is still well modeled and not degraded when contrastive learning is action-centric and an appearance-free stream is introduced. 

\subsection{Other Datasets}
To evaluate the temporality reasoning, we use Next-QA~\cite{xiao2021next}, TGif-QA~\cite{li2016tgif}, and MSRVTT-QA~\cite{xu2016msr} as benchmarks. We select the datasets based on the portion of the temporality-related questions. In Next-QA, $53\%$ contains temporal syntaxes, as mentioned in the implementation details in the supplementary material. For TGif-QA, 4 splits are fully temporal questions and 1 split contains less than $10\%$. 
MSRVTT-QA, ActivityNet-QA~\cite{yu2019activitynet}, and MSVD~\cite{chen2011collecting} contain $25\%$, $12\%$, and $8\%$ temporal questions respectively. Considering a fair comparison with SoTA VGT and our limited computation resources as well, we use Next-QA and TGif-QA's 4 splits for MC-QA evaluation and MSRVTT-QA and TGif-FrameQA for OE-QA evaluation.   

\subsection{Ablation Study on Appearance-free stream.}
In addition to Table 4-c in the main paper, Table~\ref{tab:as_app_spp} also shows that the flow maps are helpful when accompanied by the corresponding RGB frames. Motions in VideoQA cannot be extracted purely from an appearance-free stream, since appearance also provides important cues. The table also shows that with the number of clips as per video $K=16$, we achieve the best accuracy which is $57.03\%$ on test split. The accuracy slightly drops if we distributed the videos into clips that are more e.g. $K=24$ or less e.g. $K=8$. This shows that sampling at a certain rate can encode the informative features across multiple visual modalities. But beyond a certain extent of sampling rate, the model may perform worse due to overfitting. 

\begin{table}[h]
\centering
\caption{Ablation study on appearance-free stream.}
\resizebox{0.5\columnwidth}{!}{%
\begin{tabular}{l|ccc}
\toprule
Text Input  & Val ~(\%) & Test~(\%)    \\ \hline
Ours (TSN, $K=16$)  & \textbf{58.27} & \textbf{57.03}         \\ \hline
TSN-Flow only    & 56.89 & 55.85          \\ 
I3D-Flow only    & 56.76 & 55.73         \\ 
\hline
$K=8$      & 57.63 & 56.66        \\ 
$K=24$    & 57.82 & 56.35       \\ 
\bottomrule
\end{tabular}
}

\label{tab:as_app_spp}
\end{table}

\section{Additional Qualitative Analysis}
We provide more qualitative results in Figure~\ref{fig:visual_supp}.
We observe that ATM also avoids over-exploiting language bias, as the proposed AcCL helps ground the action text to the visual evidence e.g. ``baby bite'' in(1), while others may rely on the question-answer shortcuts between ``move finger to baby'' and ``a2. play with him''.

ATM focus on action modeling and it may fall short in reasoning about the object characteristics, \eg the ``light screen'' causes the girl in a ``bright face'' in (2).
Large-scale vision-language pre-training augmented with knowledge could be helpful. We leave the knowledge-driven action modeling for future work.
% \section{Other Analysis}

\section{Limitations}
While \methodname outperforms the existing methods, there is ample room for improvement. 
Although \methodname can deal with arbitrary-length video, it divides the video into a finite number of clips and extracts features per clip. This may not be adequate to capture enough action information when the action occurs in a very short time over a long duration video. 
Another challenge is time complexity of optical flow computation. It would be worthwhile to investigate efficient ways to extract the appearance-free stream.
